# Supplementary material for: When Representative Samples Produce Worse Outcomes: Scale-up Decisions and Testing in Small-Budget RCTs
Source: arXiv:2606.13531 source file (2026-06-11)
Supplement: Supplementary file 1 [file appendix-toc.tex]

\makeatletter
\newif\ifappendixcontentsactive
\appendixcontentsactivefalse

\let\appendixcontents@origaddcontentsline\addcontentsline
\renewcommand{\addcontentsline}[3]{%
  \appendixcontents@origaddcontentsline{#1}{#2}{#3}%
  \ifappendixcontentsactive
  \def\appendixcontents@ext{#1}%
  \def\appendixcontents@toc{toc}%
  \def\appendixcontents@unit{#2}%
  \def\appendixcontents@section{section}%
  \ifx\appendixcontents@ext\appendixcontents@toc
  \ifx\appendixcontents@unit\appendixcontents@section
  \appendixcontents@origaddcontentsline{atoc}{#2}{#3}%
  \fi
  \fi
  \fi
}

\newcommand{\printappendixcontents}{%
  \@ifclassloaded{acmart}{%
    \@starttoc{atoc}{Appendix Contents}%
  }{%
    \section*{Appendix Contents}%
    \@starttoc{atoc}%
  }%
  \appendixcontentsactivetrue
}

\makeatother
